# Supplementary material for: Electrically induced angular momentum flow between separated ferromagnets
Source: arXiv:2311.05290 ancillary file (2023-11-09)
Supplement: Supplementary file 1 [file Supplements.pdf]

# Supplemental Material: Electrically induced angular momentum flow between separated ferromagnets

Richard Schlitz,[1,*] Matthias Grammer,[2,3] Tobias Wimmer,[2,3] Janine Gückelhorn,[2,3] Luis Flacke,[2,3] Sebastian T.B. Goennenwein,[4] Rudolf Gross,[2,3,5] Hans Huebl,[2,3,5] Akashdeep Kamra,[6] and Matthias Althammer[2,3,†]

[1]*Department of Materials, ETH Zürich, 8093 Zürich, Switzerland*

[2]*Walther-Meißner-Institut, Bayerische Akademie der Wissenschaften, 85748 Garching, Germany*

[3]*Physics Department, TUM School of Natural Sciences, Technische Universität München, 85747 Garching, Germany*

[4]*Department of Physics, University of Konstanz, 78457 Konstanz, Germany*

[5]*Munich Center for Quantum Science and Technology (MCQST), 80799 München, Germany*

[6]*Condensed Matter Physics Center (IFIMAC) and Departamento de Física Teórica de la Materia Condensada, Universidad Autónoma de Madrid, E-28049 Madrid, Spain*

(Dated: November 9, 2023)

## SAMPLE FABRICATION AND CONNECTION SCHEME FOR ELECTRICAL TRANSPORT MEASUREMENTS

### Sample fabrication

We fabricated electrical transport device structures on top of (111)-oriented yttrium aluminium garnet ($Y_3Al_5O_{12}$, YAG) or (0001)-oriented sapphire ($Al_2O_3$) substrates using electron beam lithography and lift-off techniques or etching of the plain thin films. Each device consists of two metal strips with strip width $w$, a strip edge-to-edge separation $d$, and a length of $l = 100\ \mu$m. For the metal strips we used Ni(10-20), Co(10), $Co_{25}Fe_{75}$(7)[CoFe], $Ni_{80}Fe_{20}$(5-20)[Py], Pt(4) deposited via electron beam evaporation or sputtering, the values in parenthesis are the respective thickness values in nm. To avoid oxidization of the FM we capped those layers with a 3 nm thin Al layer. In addition, we fabricated 4 strip structures consisting of two CoFe(7) strips and two $Ni_{80}Fe_{20}$(7)[Py] strips, with the same edge-to-edge separation between each strip and the same width. Subsequently, Al contact structures are deposited via sputtering.

In the following, we provide the dimensions and measurement currents of the respective devices used in the experiments:

- Ni-Ni: $t_{\mathrm{Ni}} = 10$ nm, $d = 50$ nm, $w = 1\ \mu$m, $I_{\mathrm{inj}} = 200\ \mu$A on YAG,
- CoFe-Py: $t_{\mathrm{CoFe,Py}} = 7$ nm, $d = 300$ nm, $w = 1\ \mu$m, $I = 500\ \mu$A on YAG,
- Py-Py(15): $t_{\mathrm{Py}} = 15$ nm, $d = 50$ nm, $w = 1\ \mu$m, $I_{\mathrm{inj}} = 500\ \mu$A on YAG,
- Py-Py(10): $t_{\mathrm{Py}} = 10$ nm, $d = 50$ nm, $w = 1\ \mu$m, $I_{\mathrm{inj}} = 500\ \mu$A on YAG,
- Py-Py(7): $t_{\mathrm{Py}} = 7$ nm, $d = 300$ nm, $w = 1\ \mu$m, $I_{\mathrm{inj}} = 500\ \mu$A on YAG,
- Py-Py(5): $t_{\mathrm{Py}} = 5$ nm, $d = 50$ nm, $w = 1\ \mu$m, $I_{\mathrm{inj}} = 500\ \mu$A on YAG,
- Py-Py $Al_2O_3$: $t_{\mathrm{Py}} = 7$ nm, $d = 50$ nm, $w = 1\ \mu$m, $_{\mathrm{inj}} = 500\ \mu$A on $Al_2O_3$,
- CoFe-CoFe: $t_{\mathrm{CoFe}} = 7$ nm, $d = 300$ nm, $w = 1\ \mu$m, $I_{\mathrm{inj}} = 500\ \mu$A on YAG,
- Ni-Py: $t_{\mathrm{Ni,Py}} = 20$ nm, $d = 50$ nm, $w = 1\ \mu$m, $I_{\mathrm{inj}} = 500\ \mu$A on YAG,
- Py-Ni: $t_{\mathrm{Ni,Py}} = 20$ nm, $d = 300$ nm, $w = 1\ \mu$m, $I_{\mathrm{inj}} = 500\ \mu$A on YAG,
- CoFe-Pt: $t_{\mathrm{CoFe}} = 7$ nm, $t_{\mathrm{Pt}} = 4$ nm, $d = 400$ nm, $w = 250$ nm, $I_{\mathrm{inj}} = 100\ \mu$A on YAG,

**Electrical measurement scheme**

The fabricated samples have been mounted into superconducting magnet cryostats equipped with a 3d vector magnet (maximum magnetic field 2.5 T) or a split-coil magnet (maximum magnetic field 7 T) with a rotatable sample stage. Electrical transport measurements were conducted via a dc charge current bias and voltage detection via nanovoltmeters. We illustrate our connection scheme that has been used consistently for all our electrical measurements in Fig. S1. For the investigation of the transport properties in our two-strip devices, we perform angle-dependent measurements. The orientation of an external magnetic field $\mathbf{H}$ with constant magnitude $\mu_0 H$ is varied in three distinct rotation planes illustrated in the main text. For each field orientation we apply a dc charge current with a positive and negative polarity $\pm I_{\mathrm{inj}}$ to one metal strip (injector), while we measure the dc-voltage $V(\pm I)$ at the second metal strip (detector). Utilizing this current reversal method, we are able to separate contributions even (thermal signals, $V_{\mathrm{therm}}$) and odd (resistive signal, $V_{\mathrm{det}}$) with respect to the charge current polarity [1]:

$$V_{\mathrm{therm}} = (V(+I_{\mathrm{inj}}) + V(-I_{\mathrm{inj}}))/2\,, \tag{S1}$$

$$V_{\mathrm{det}} = (V(+I_{\mathrm{inj}}) - V(-I_{\mathrm{inj}}))/2\,. \tag{S2}$$

We attribute the origin of $V_{\mathrm{therm}}$ to Joule heating induced by the charge current applied to the injector (see discussion below), while $V_{\mathrm{det}}$ at the detector is caused by effects scaling linearly with $I$. The observed angle-dependence of $V_{\mathrm{therm}}$ is well explained by the contributions of temperature gradients driven by the Joule heating in the injector strip and accounting for the different magnetothermopower effects (see discussion below). We note that $V_{\mathrm{det}}$ is calculated directly from the measurement data and we did not subtract any offset voltage to avoid any ambiguities. Moreover, we varied the delay time between switching the current polarity and triggering the voltage readout by up to 3 s and found no significant changes in the voltage signal.

From the angle-dependent $V_{\mathrm{det}}$ signals, we extract the amplitude $\Delta V_{\mathrm{det}}$ from a $\cos^2(\beta, \gamma)$-fit to the data to increase the number of datapoints contributing to this value. Error bars given for $\Delta V_{\mathrm{det}}$ are determined using this fitting procedure.

## FIT PARAMETERS FOR THE DISTANCE DEPENDENT MEASUREMENT DATA

We summarize in Tab. S1 the obtained fit parameters by fitting Eq. (1) of the main text to our distance dependent Py-Py data.

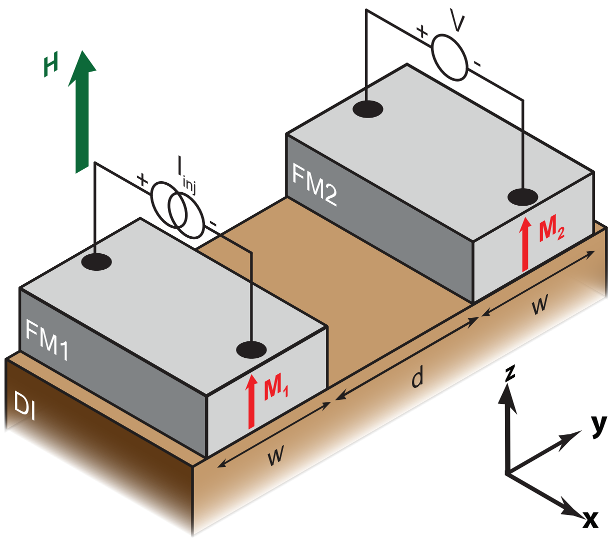


FIG. S1. Illustration of the contact scheme used for the measurements to define injected charge current polarity and detected voltage polarity.

| Sample | $c_1$ | $c_2$ |
|---|---|---|
| Py-Py(15) | $7.8 \pm 0.2 \times 10^{-6}$ | $197 \pm 1$ nm |
| Py-Py(10) | $2.7 \pm 0.4 \times 10^{-6}$ | $290 \pm 60$ nm |
| Py-Py(5) | $9.5 \pm 0.5 \times 10^{-7}$ | $170 \pm 20$ nm |
| Py-Py $Al_2O_3$ | $1.7 \pm 0.3 \times 10^{-6}$ | $330 \pm 90$ nm |

TABLE S1. Results obtained from fitting the distance dependence in the main text.

## THERMAL TRANSPORT SIGNALS

In Fig. S2, we show $V_{\text{therm}}$ obtained for our four devices with different metal strips in the three orthogonal rotation planes ip, oopj and oopt of **h** [see Fig. 1(e-g) in the main text for a sketch of the rotation planes]. For all four structures we find a $\cos(\beta,\gamma)$-dependence for the oopj and oopt rotation planes with maxima and minima when **h** is oriented in the out-of-plane direction (0°, 180°). We attribute these signals to the anomalous Nernst effect for the Ni-Ni, Co-Co, CoFe-CoFe samples and the ordinary Nernst effect in case of the Pt-Pt sample. These thermal voltage signals are induced by the in-plane thermal gradient along the **t**-direction originating from the Joule heating at the injector. Interestingly, the angle-dependence is inverted for the Co-Co structure, which can be explained by a sign inversion of the anomalous Nernst angle. Yet, due to the fact

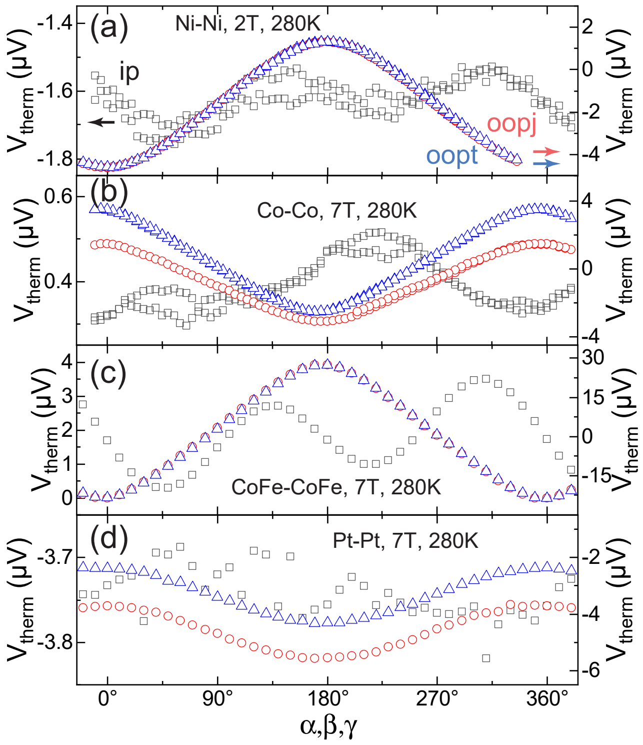


FIG. S2. (a)-(d) Angle-dependent $V_{\mathrm{therm}}$ signals measured at 280 K and $\mu_0 H = 2$ T/7 T for (a) Ni-Ni strips ($d = 50$ nm, $w = 1$ $\mu$m, $I_{\mathrm{inj}} = 200$ $\mu$A), (b) Co-Co strips : ($d = 50$ nm, $w = 1$ $\mu$m, $I_{\mathrm{inj}} = 200$ $\mu$A), (c) CoFe-CoFe strips ($d = 400$ nm, $w = 250$ nm, $I_{\mathrm{inj}} = 100$ $\mu$A), and (d) Pt-Pt strips ($d = 400$ nm, $w = 250$ nm, $I_{\mathrm{inj}} = 200$ $\mu$A). Black squares correspond to ip-rotations, red circles to oopj-rotations and blue triangles to oopt rotations. Left y-scale for ip-rotations, right y-scale for oopj and oopt rotations.

that FM thin films exhibit a complex thickness dependence of the anomalous Nernst angle [2], we cannot directly attribute this sign inversion to the corresponding bulk material properties. The amplitude of the $\cos(\beta, \gamma)$ angle dependence increases with increasing field and saturates for large magnetic fields for the three ferromagnetic samples, while it increases linearly with $\mu_0 H$ for the Pt-Pt sample, further supporting our assumed anomalous Nernst and Nernst effect origin of the observed signals (data not shown) [3].

The Ni-Ni, Co-Co, and CoFe-CoFe samples exhibit a systematic angle-dependence for the ip rotation plane. We attribute the observed evolution with the external magnetic field orientation in the FM detectors to two contributions: the transverse anisotropic magnetothermopower, also referred to as the planar Nernst effect, [4–7] and an additional $\cos(\alpha)$ dependence due to contributions from the anomalous Nernst effect. The transverse anisotropic magnetothermopower is induced by the in-plane temperature gradient in the FM detector strip and exhibits a $\cos(\alpha)\sin(\alpha)$

angle dependence with maxima at 45°, 225° and minima at 135°, 315°. The superimposed $\cos(\alpha)$ angle-dependence by the anomalous Nernst effect can be either attributed to an imperfect sample alignment with an out-of-plane magnetic field component for the ip-rotations (driven by the in-plane temperature gradient along **t**) or may also originate from an additional out-of-plane temperature gradient in the FM detector. In principle, these two contributions could be disentangled by evaluating the magnetic field dependence of this $\cos(\alpha)$ contribution. Unfortunately, the superimposed contribution from the transverse anisotropic magnetothermopower and the noise in our measurements prevents a solid conclusion from such an analysis.

We note that we refrain from a quantitative comparison of $V_{\text{therm}}$ between samples and rotation planes, since this requires exact quantitative knowledge of the temperature profile present in the different samples, which is very difficult to obtain.

## ADDITIONAL ANGLE-DEPENDENT EXPERIMENTS

We plot further angle-dependent data obtained with different combinations of ferromagnetic metals and platinum strips in Fig. S3. The different constant offset voltages for the different rotation planes are attributed to the necessary sample remounting for each rotation plane and corresponding small leakage currents flowing in the wiring of the measuring insert.

For all FM1-FM2 combinations we observe a $\cos^2(\beta,\gamma)$-dependence for the oopj and oopt rotation planes and no angle-dependence for the ip rotation plane [see Fig. S3(a-d)]. This indicates that the observed effect is indeed universal and occurs for many different ferromagnetic metals. The strength of the effect seems to be not affected if two materials with large differences in saturation magnetization, like for example CoFe and Py, are used, as evident from Fig. S3(c).

A possible other mechanism beyond dipolar coupling and phononic angular momentum transport would be electromagnetic coupling of thermal fluctuations and spin-rectification via the anomalous Hall effect (AHE) due to the applied charge current bias. The AHE-based spin rectification relies on magnetic fluctuations that are coherently coupled between the two FMs by dipolar interactions and the fact that charge fluctuations can bridge the gap between the two wires by capacitive/inductive coupling. With these two assumptions, the AHE can give rise to a DC voltage signal in the detector by rectification. The voltage sign measured at the detector strip will then depend on the sign of the AHE coefficient in both FMs and is negative for two materials with opposite sign in the AHE coefficient. We therefore perform experiments [see Fig. S3(d)] on wires

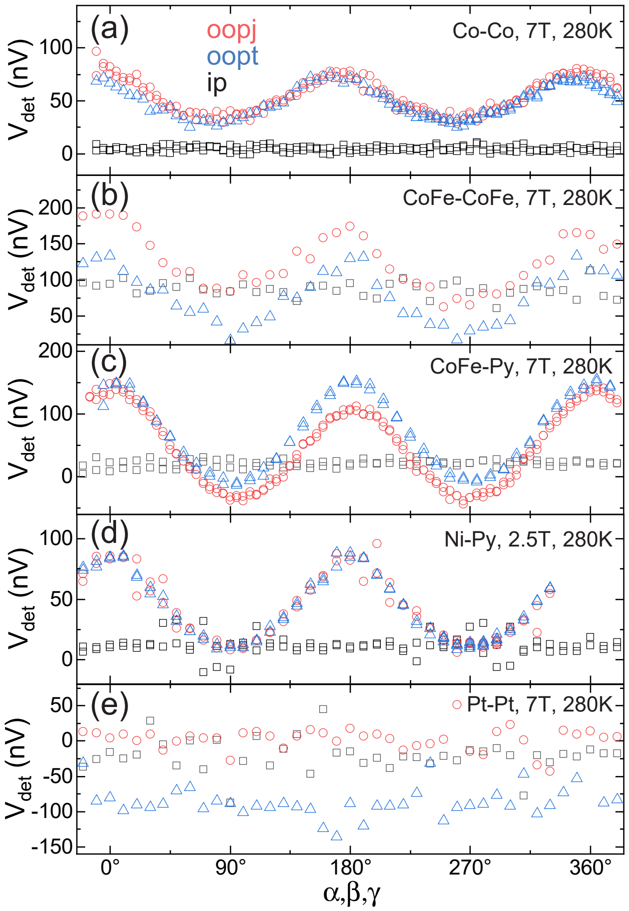


FIG. S3. Angle-dependence of $V_{\mathrm{det}}$ for (a) Co-Co strips , (b) CoFe-CoFe strips , (c) CoFe-Py strips , (d) Ni-Py strips. and (e) Pt-Pt strips measured at 280 K and $\mu_0 H = 2.5, 7$ T. Black squares correspond to ip-rotations, red circles to oopj-rotations and blue triangles to oopt rotations, respectively.

of Ni and Py, having AHE of opposite sign (see below for extraction of the AHE polarity for our thin films) [8] to show that the sign of the modulation is not inverted. This observation, together with the observation of the effect for ferromagnets with mismatched saturation magnetization excludes a potential influence of this mechanism.

We do not observe any angle-dependence for $V_{\mathrm{det}}$ if both (or one, see main text) strips are made of Pt [see Fig. S3(e)]. This indicates that the magnetic order and associated magnons of the metal strips are key in observing the effect in the experiment.

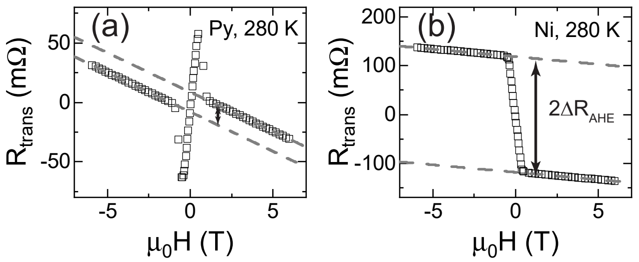


FIG. S4. Anomalous Hall effect measurements for Ni and Py layers using a Hallbar structure ($t_{\mathrm{Py}} = t_{\mathrm{Ni}} =$ 20 nm). Field-dependence of the transverse resistance for (a) Py and (b) Ni. The grey dashed lines indicate the linear fits used to extract

## SIGN OF THE ANOMALOUS HALL EFFECT

To confirm that the sign of the AHE is indeed opposite for the Py and Ni layers, we measured the transverse voltage response in a Hallbar structure on the same chip as the angular momentum transport structures. Utilizing the current reversal technique and extracting the antisymmetric component of the signal with respect to magnetic field inversion, we obtained the results shown in Fig. S4 at $T = 280$ K.

From the linear fit to the data in the high field limit (dashed grey lines) we extract the AHE resistivity $\rho_{\mathrm{AHE}} = R_{\mathrm{AHE,Py/Ni}} t_{\mathrm{Py/Ni}}$ for both materials from the intercept [8]. We obtain $\rho_{\mathrm{AHE}} = -2.4$ nΩm for Ni and $\rho_{\mathrm{AHE}} = +0.17$ nΩm for Py, these values agree well with the results obtained in Ref. [8]. Most importantly, they show that the sign of the AHE is opposite for Ni and Py.

## FOUR STRIP DEVICES

As a final step we looked into the detector voltages obtained for a four strip device consisting of two CoFe and two Py strips (with identical $d = 300$ nm, $w = 1$ $\mu$m), as indicated by the illustrations in Fig. S5. We only observe an angle dependence of $V_{\mathrm{det}}$ for the oopj and oopt rotation planes. In Fig. S5 we plot the voltages measured for two different driving schemes, once the charge current is applied to the inner CoFe strip and in the other case to the inner Py strip for the oopj rotation plane. In the naming scheme we note down the driven FM strip (CoFe2 or Py1) followed by the strip where the voltage $V_{\mathrm{det}}$ was detected, for example CoFe2-Py1.

In this rotation plane we observe for the three simultaneously measured voltages a roughly $\cos^2(\beta,\gamma)$-dependence of $V_{\mathrm{det}}$, consistent with our experiments with two FM strips. The amplitude

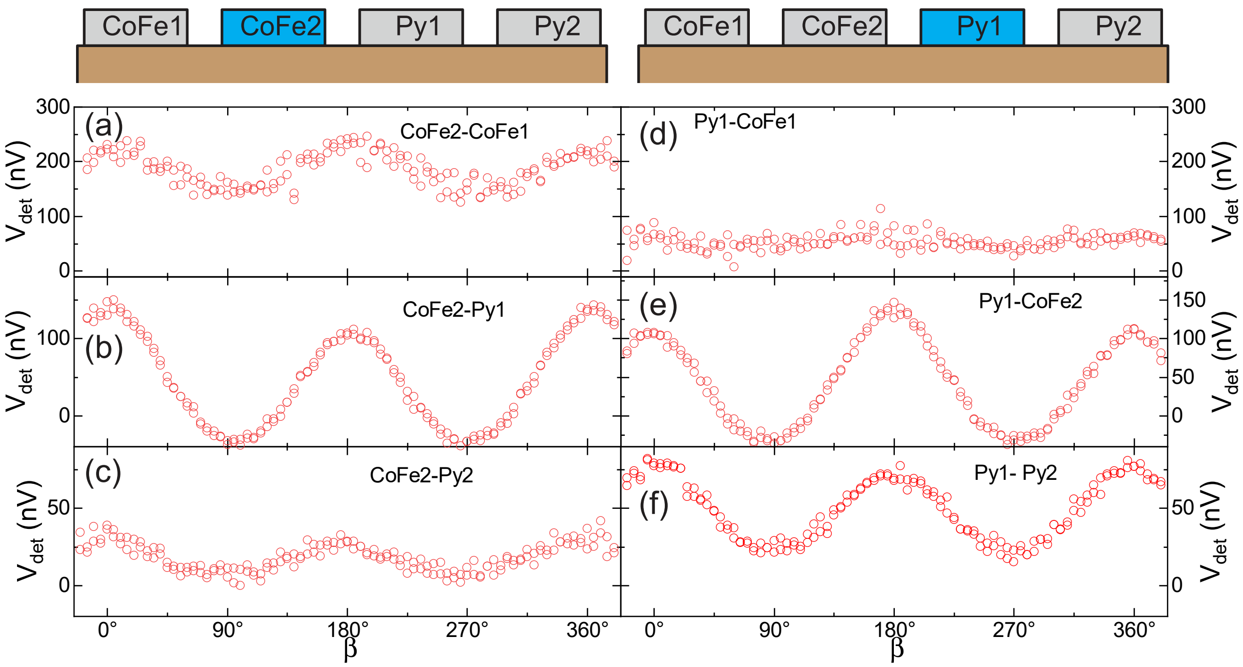


FIG. S5. Detector voltages for a 4 strip device ($d$ = 300 nm, $w$ = 1 $\mu$m, $I$ = 500 $\mu$A) consisting of 2 different FMs, CoFe and Py (as shown by the illustrations above) for an oopj rotation at 7 T and 280 K. (a)-(c) Angle-dependent voltages measured at the outer CoFe strip (CoFe1), inner Py strip (Py1) and outer Py strip (Py2) when driving the charge current through the inner CoFe strip (CoFe2). (d)-(f) $V_{\mathrm{det}}(\beta)$ at the outer CoFe strip (CoFe1), inner CoFe strip (CoFe2) and outer Py strip (Py2) when driving the charge current through the inner Py strip (Py1).

of this $\cos^2(\beta,\gamma)$-dependence varies for all strips and is the largest for the two inner different FM strips. Moreover, a maximum in $V_{\mathrm{det}}$ is obtained for $\mathbf{m} \parallel \pm\mathbf{z}$, in agreement with the previous results with two FM strips. We note that for the applied external magnetic field of 7 T it is safe to assume that the magnetization in all 4 strips is aligned parallel to the external magnetic field. From these experiments we can further strengthen the conclusion, that also two strips with different FMs give rise to the observed out-of-plane angle-dependence. Moreover, the angle-dependence persists even for the outer strips, where an additional FM strip is in between the FM strip at which the charge current is applied to.

In Fig. S5(b) and (e), we switched the role of the two inner FM strips, and find a remarkable violation of reciprocity. For CoFe2-Py1, the maxima at 0° and 360° are higher than the maximum at 180°, in contrast for Py1-CoFe2 the it is the other way around the maxima at 0° and 360° are lower than the maximum at 180°. For the other two mixed configurations CoFe2-Py2 and Py1-

CoFe1, the noise makes it difficult to verify any 180° asymmetry in the angle-dependence. At present we have no immediate explanation of this non-reciprocity and can only speculate about the origin. Interestingly, a similar nonreciprocity was also found in magnon transport experiments with ferromagnetic electrodes on a magnetic insulator [9].

* richard.schlitz@mat.ethz.ch

† matthias.althammer@wmi.badw.de

[1] M. Schreier, N. Roschewsky, E. Dobler, S. Meyer, H. Huebl, R. Gross, and S. T. B. Goennenwein, Current heating induced spin seebeck effect, Applied Physics Letters **103**, 242404 (2013).

[2] T. C. Chuang, P. L. Su, P. H. Wu, and S. Y. Huang, Enhancement of the anomalous Nernst effect in ferromagnetic thin films, Physical Review B **96**, 174406 (2017).

[3] J. Gao, C.-H. Lambert, R. Schlitz, M. Fiebig, P. Gambardella, and S. Vélez, Magnon transport and thermoelectric effects in ultrathin $Tm_3Fe_5O_{12}$/Pt nonlocal devices, Phys. Rev. Res. **4**, 043214 (2022).

[4] V. D. Ky, The planar Nernst effect in permalloy films, physica status solidi (b) **17**, K207 (1966).

[5] V. D. Ky, Planar Hall and Nernst effect in ferromagnetic metals, physica status solidi (b) **22**, 729 (1967).

[6] Y. Pu, E. Johnston-Halperin, D. D. Awschalom, and J. Shi, Anisotropic thermopower and planar Nernst effect in $Ga_{1-x}Mn_xAs$ ferromagnetic semiconductors, Physical Review Letters **97**, 036601 (2006).

[7] A. D. Avery, M. R. Pufall, and B. L. Zink, Observation of the planar Nernst effect in permalloy and nickel thin films with in-plane thermal gradients, Physical Review Letters **109**, 196602 (2012).

[8] Y. Omori, E. Sagasta, Y. Niimi, M. Gradhand, L. E. Hueso, F. Casanova, and Y. Otani, Relation between spin Hall effect and anomalous Hall effect in 3d ferromagnetic metals, Physical Review B **99**, 014403 (2019).

[9] T. Wimmer, B. Coester, S. Geprägs, R. Gross, S. T. B. Goennenwein, H. Huebl, and M. Althammer, Anomalous spin hall angle of a metallic ferromagnet determined by a multiterminal spin injection/detection device, Applied Physics Letters **115**, 092404 (2019).
